# Supplementary material for: Causality in Video Diffusers is Separable from Denoising
Source: arXiv:2602.10095 source file (2026-02-10)

Block 15

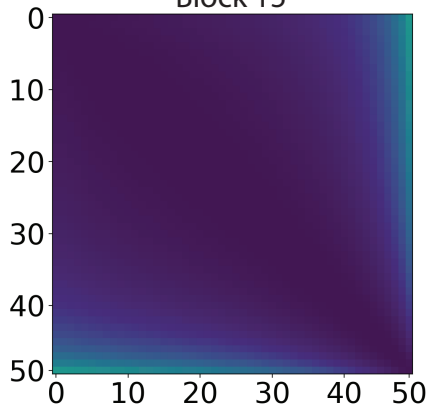

Block 20

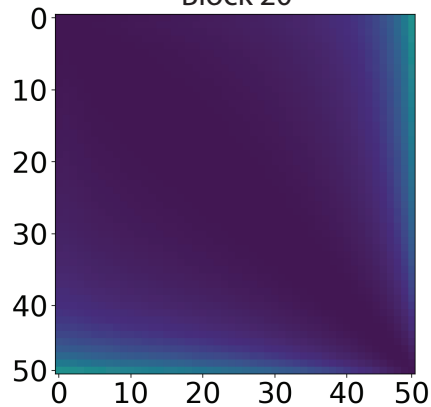

Block 25

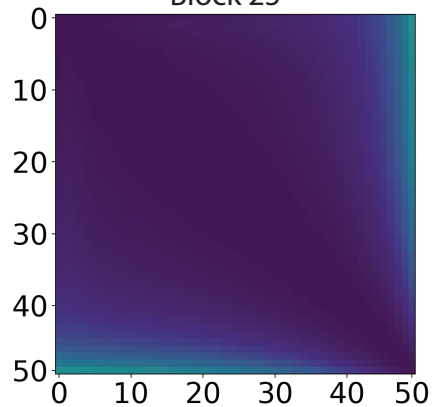

Block 27

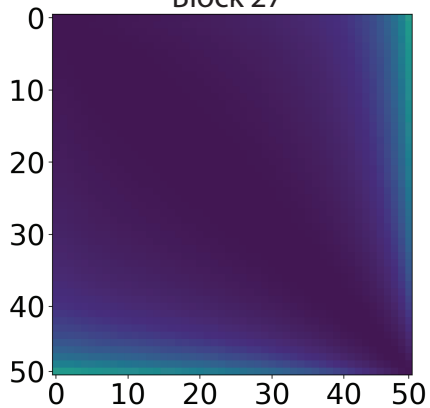

Block 28

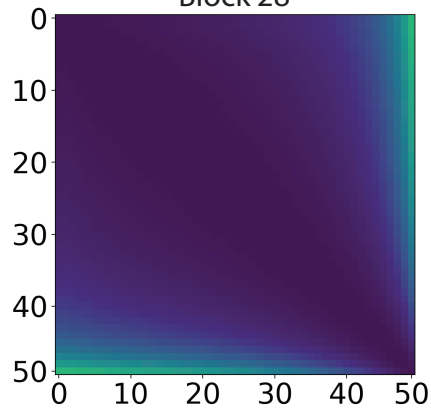

Block 29

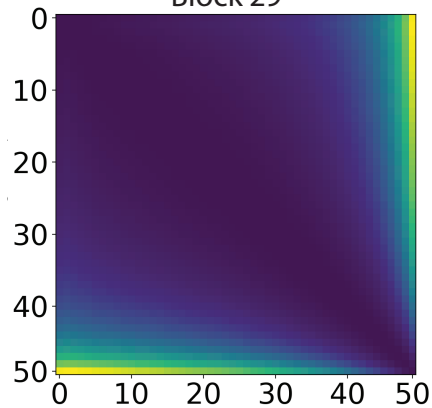

MSE distance (avg per pixel)

Block 27

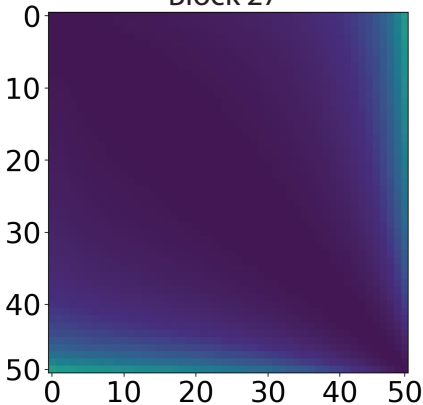

Supplement: Supplementary file 1 [file sf_similarity.pdf]
